# Supplementary material for: Rapid multiplex ultrafast nonlinear microscopy for material characterization
Source: arXiv:2208.06633 ancillary file (2022-08-13)
Supplement: Supplementary file 1 [file OpticsExpress_SI_v2.pdf]

## 1. PULSE COMPRESSION SETUP

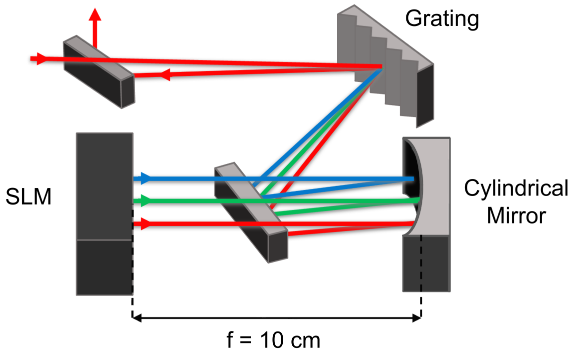


**Fig. S1.** Schematic drawing of SLM-based pulse shaper used to compress pulses utilized for the experiments presented in the main text.

The spatial light modulator (SLM)-based pulse shaper employed in our setup is shown in Fig. S1. The pulse compression setup was adapted from the design presented in Ref.[1]. This setup compensates for the large amounts of nonlinear dispersion accumulated from optical elements utilized in the ultrafast nonlinear imaging setup presented in the main text. The laser pulses are spatially dispersed using a 1200 grooves/mm grating and focused onto the SLM using a 10 cm focal length cylindrical mirror. These optics have been chosen to spread the laser spectrum across a large number of pixels on the SLM, mitigating detrimental effects of pixelation and cross-talk between adjacent pixels on the compressed pulses. The SLM (Meadowlark Optics 1x12K Linear SLM) then acts as a variable phase mask and is used to alter the phase of individual wavelengths of the laser spectrum.

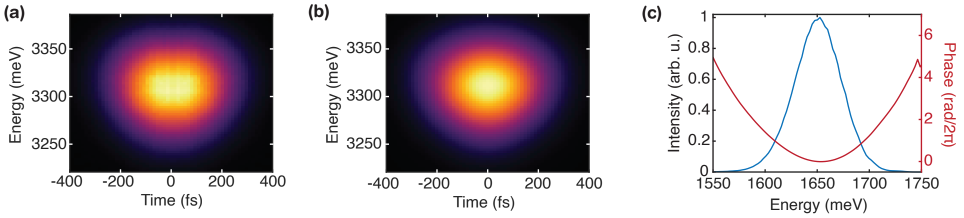


**Fig. S2.** **(a)** Measured FROG trace of the reference pulse. **(b)** Reconstructed FROG trace of the reference pulse. **(c)** Reconstructed spectrum and spectral phase of the reference pulse.

We employ phase-resolved cross correlation with a known reference pulse. We interfere the reference pulse with the signal pulse and generate a reference for the phase-resolved measurement as follows: After combining the two pulses, we split of half the signal using a beamsplitter and spectrally narrow it using a grating and thin slit before sending the beams onto a detector. This ensures a reference that is temporally longer lived than the signal. This is similar to the procedure employed in [2] for generating a reference signal. The reference signal is subsequently electronically processed with the procedure outlined in [3] and can be efficiently filtered out by exploiting the beat note between the amplitude modulation that the laser repetition rate imparts on the reference pulse, and the amplitude modulation imparted on the signal pulse by an acousto-optic modulator. The other half of the signal is sent directly onto a detector and used as the lock-in input. By scanning the delay between reference and signal pulse, we obtain full amplitude and phase information in the temporal domain and, by Fourier transform, can obtain spectral amplitude and phase information of our laser pulse. The reference pulse is characterized using Second-harmonic generation Frequency-resolved optical gating (SHG-FROG). The measured and reconstructed FROG trace are shown in Fig. S2(a,b). The corresponding spectrum and spectral phase of the reference pulse is shown in Fig. S2(c).

We present spectral amplitude and phase information of our signal laser pulses measured at the sample position (in the following: signal pulse) in Fig. S3(a). Within the bandwidth of

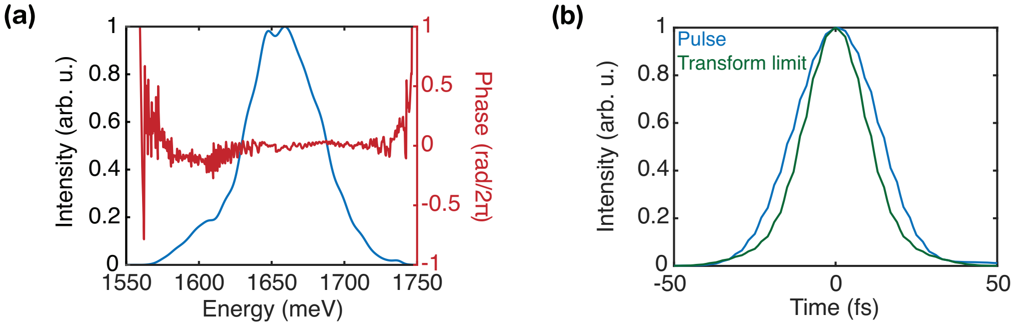


**Fig. S3.** **(a)** Laser pulse spectrum and corresponding phase and **(b)** time domain trace and transform limited pulse of the laser spectrum.

our laser, the complex phase is shown to be mostly flat, supporting that much of the dispersion has been corrected for by the pulse compression system. In Fig. S3(b) we show the compressed pulse together with its transform limit in the temporal domain. Fitting the time domain traces to Gaussian pulses, we determine the full width half maximum (FWHM) of the laser pulse to be 30 fs as compared to the FWHM of 24 fs for the transform limit, suggesting we have near-transform limited pulses.

## 2. FINITE PULSE EFFECTS

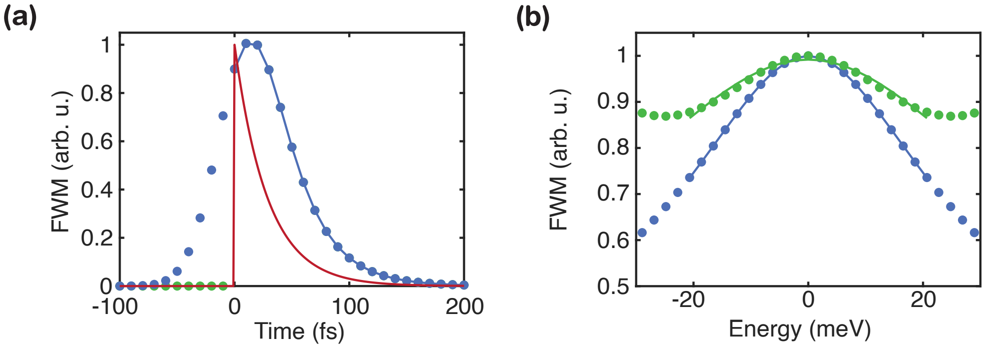


**Fig. S4.** **(a)** Dephasing curve with $T_2 = 30$ fs without finite pulse effects (red) and with finite pulse effects for a 20 fs pulse (blue curve). **(b)** Lineshape retrieved from the blue curve in (a) after considering the finite bandwidth from finite pulse effects (blue), and retrieved from the green curve in (a) where all signal at negative times is set to zero.

Despite efficient pulse compression, when the pulse duration $T_{\text{pulse}}$ approaches the time-scales of the sample dynamics such as dephasing time $T_2$ or population decay time $T_1$, finite pulse effects influence the retrieved dynamics of the sample. This is evident from Fig. S4(a), where we plot the simulated sample response for 20 fs pulses to a dephasing process with a dephasingtime $T_2 = 30$ fs. The pure sample response (red) does not consider finite pulse effects while the actual response (blue) takes them into account. We also show a fit function taking the finite pulse effects into account (blue solid line). The effects of finite pulse effects on the sample response differs for the different modalities presented in the main text. For population scans, the sample response is modeled by convolving an exponential decay with the cross correlation of the intensities of the pump and probe pulses [4]. For dephasing maps, the same procedure as for multi-dimensional coherent spectroscopy (MDCS) needs to be employed. As inferred from Ref.[5], when also considering heterodyne detection with a fourth pulse, finite pulse effects in the frequency domain correspond to finite bandwidth effects and can be considered by dividing the MDCS spectrum with the intensity spectrum of the laser pulse along the two frequency axes. Given the Gaussian shape of the spectrum, this corresponds to convolving the time-domain response along the diagonal with $E^{1/4}(t')$. Here, $E(t')$ is the Gaussian pulse profile in the temporal

domain. Considering the finite pulse effects in the frequency vs. time domain is equivalent in the idealized scenario presented here. In Fig. S4(a) the real sample response extends to negative times, Fourier transforming this response and doing a Lorentzian linewidth fit in the frequency domain after employing the spectral normalization procedure introduced above yields the same results for the dephasing time $T_2$ as the time-domain fit. The resulting lineshape and fit after considering the finite pulse effects in the frequency domain is shown in Fig. S4(b) in blue. As discussed by Ref.[6], interaction ordering of the various pulses plays an important role in multi-pulse experiments. In this scenario, negative time delays are often excluded because they contain contributions from additional signal pathways that interfere with the sample response of interest. However, this also removes the real negative time-signal in Fig. S4(a). Setting the signal to zero for negative times (green dots) yields a significantly altered lineshape in Fig. S4(b). The corresponding fit deviates from the data points and shows a significantly broadened linewidth, compared to the blue fit. The retrieved dephasing time in this scenario is $T_2$=18 fs, significantly below the true value of 30 fs. We avoid underestimating the dephasing time in our time-domain experiments and fits by considering finite pulse effects in our fit function while also only fitting datapoints for sufficiently large delay times at which interaction-ordering effects are negligible. Excluding these effects is non-trivial in the frequency domain and elucidated upon further in [6]. This is the reason for our multi-dimensional coherent imaging spectroscopy (MDCIS) measurements in the main text underestimating the retrieved dephasing times by few femtoseconds.

## 3. DECAY CURVES

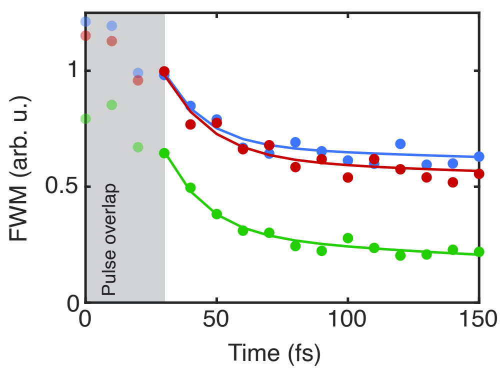


**Fig. S5.** Decay curves for $T$ delays between 0-150 fs, highlighting the rapid decay and finite pulse effects at early times.

Fig. S5 shows the decay curves from the main text in the range of 0-150 fs for the time delay $T$. Again, finite pulse effects are observable during early delay times, followed by a rapid decay. The good agreement between fit and data for early times yields reliable retrieval of exciton population decay times.

## REFERENCES


1. J. Pupeikis, N. Bigler, S. Hrisafov, C. R. Phillips, and U. Keller, "Programmable pulse shaping for time-gated amplifiers," Opt. Express **27**, 175–184 (2019).
2. P. F. Tekavec, G. A. Lott, and A. H. Marcus, "Fluorescence-detected two-dimensional electronic coherence spectroscopy by acousto-optic phase modulation," The J. Chem. Phys. **127**, 214307 (2007).
3. E. W. Martin, C. L. Smallwood, T. L. Purz, H. G. Ruth, and S. T. Cundiff, "Real-time reference for frequency-shifted fourier-transform spectrometers using an arbitrary-wavelength cw reference laser," in *2019 Conference on Lasers and Electro-Optics (CLEO)*, (2019), pp. 1–2.
4. D. Polli, D. Brida, S. Mukamel, G. Lanzani, and G. Cerullo, "Effective temporal resolution in pump-probe spectroscopy with strongly chirped pulses," Phys. Rev. A **82**, 053809 (2010).
5. C. L. Smallwood, T. M. Autry, and S. T. Cundiff, "Analytical solutions to the finite-pulse bloch model for multidimensional coherent spectroscopy," J. Opt. Soc. Am. B **34**, 419–429 (2017).

6. S. M. Gallagher Faeder and D. M. Jonas, "Two-dimensional electronic correlation and relaxation spectra: Theory and model calculations," The J. Phys. Chem. A **103**, 10489–10505 (1999).
